# Supplementary material for: Multiscale Modeling of Abnormal Grain Growth: Role of Solute Segregation and Grain Boundary Character
Source: arXiv:2510.15840 ancillary file (2025-10-26)
Supplement: Supplementary file 1 [file anc.pdf]

# Supplementary Material
# Multiscale Modeling of Abnormal Grain Growth: Role of Solute Segregation and Grain Boundary Character

Albert Linda[a], Rajdip Mukherjee*[a,], Somanth Bhowmick*[a,]

[a] *Department of Materials Science and Engineering, Indian Institute of Technology, Kanpur, Kanpur-208016, UP, India*

## 1. Diffusivity Table from Literature

| **Elements** | **Diffusivity**($\times 10^{-21}$) $m^2/s$ |
|---|---|
| Co | 2.6[1] |
| Cr | 7.1[2] |
| Mn | 19.0[3] |
| Mo | 11.1[4] |
| Nb | 11.7[5] |
| Ni | 30.0[6] |
| Ti | 29.2[7] |
| W | 4.4[8] |
| V | 50.0[9] |

Table S1: Diffusivity of elements in $\alpha$-Fe matrix at 850K, obtained from previously reported experimental results.

*Corresponding Authors

*Email addresses:* `rajdipm@iitk.ac.in` (Rajdip Mukherjee*), `bsomnath@iitk.ac.in` (Somanth Bhowmick*)

## 2. Segregation energy vs. Voronoi volume for different GB sites

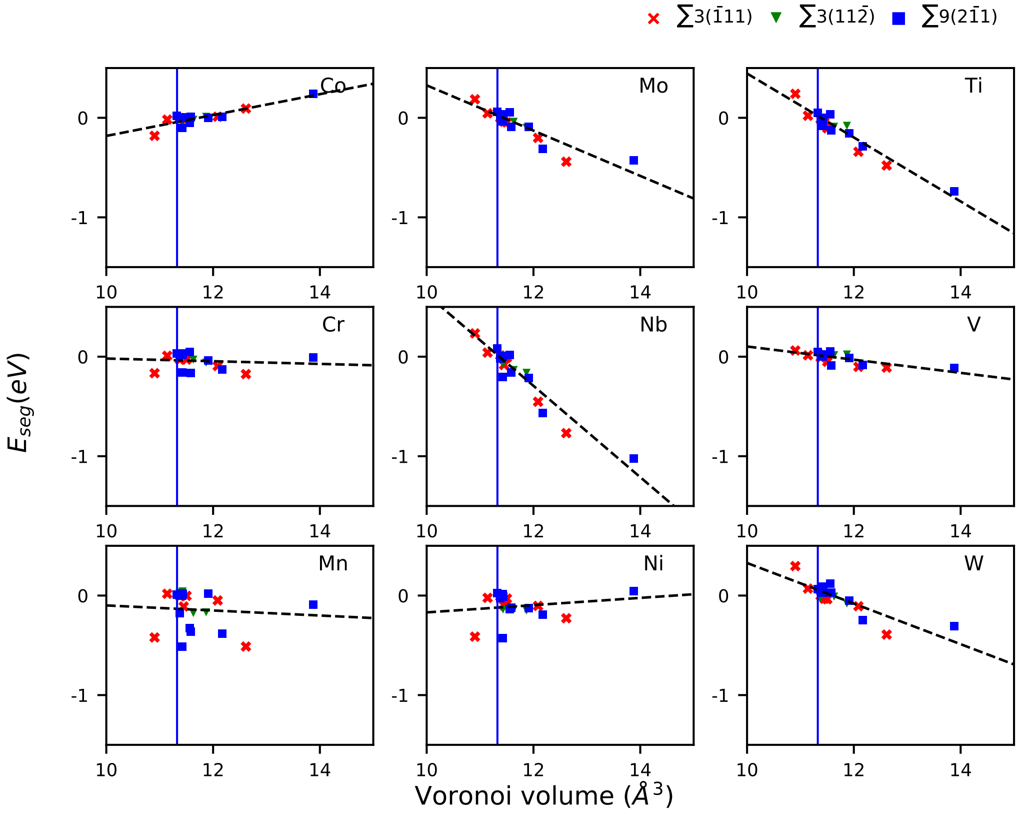


Figure S1: Plot of segregation energy vs. Voronoi volume for different GB sites. The vertical line marks the Voronoi volume of bulk Fe. For most of the cases, higher the difference of Voronoi volume between GB and bulk sites, more is the magnitude of $E_{seg}$ values. This explains the general trend of relatively small $E_{seg}$ values in case of low energy $\Sigma3(11\overline{2})$, compared to the other two grain boundaries considered in this work.

## 3. Grain boundary concentration

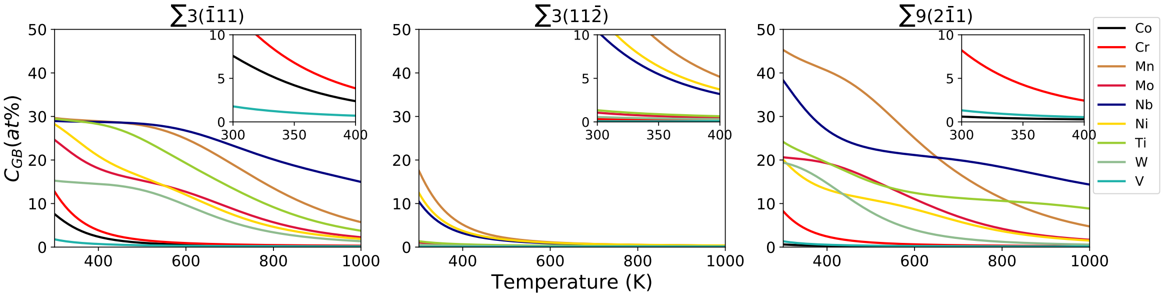


Figure S2: Variation in GB concentration with temperature, derived from the multisite McLean isotherm using a bulk solute concentration of 0.1%.

For a particular solute atom, the GB concentration for a multisite segregation can be obtained by taking the sum of all sites:

$$C_{\mathrm{GB}} = \frac{1}{n} \sum_{i}^{n} \frac{C_b \exp(-E^i_{\mathrm{seg}}/k_B T)}{1 - C_b + C_b \exp(-E^i_{\mathrm{seg}}/k_B T)} \tag{1}$$

Here $E^i_{\mathrm{seg}}$ is the segregation energy for site $i$, $C_b$ is the bulk concentration and $n$ is the number of sites. The plot for multisite GB concentration is shown in Figure S2.

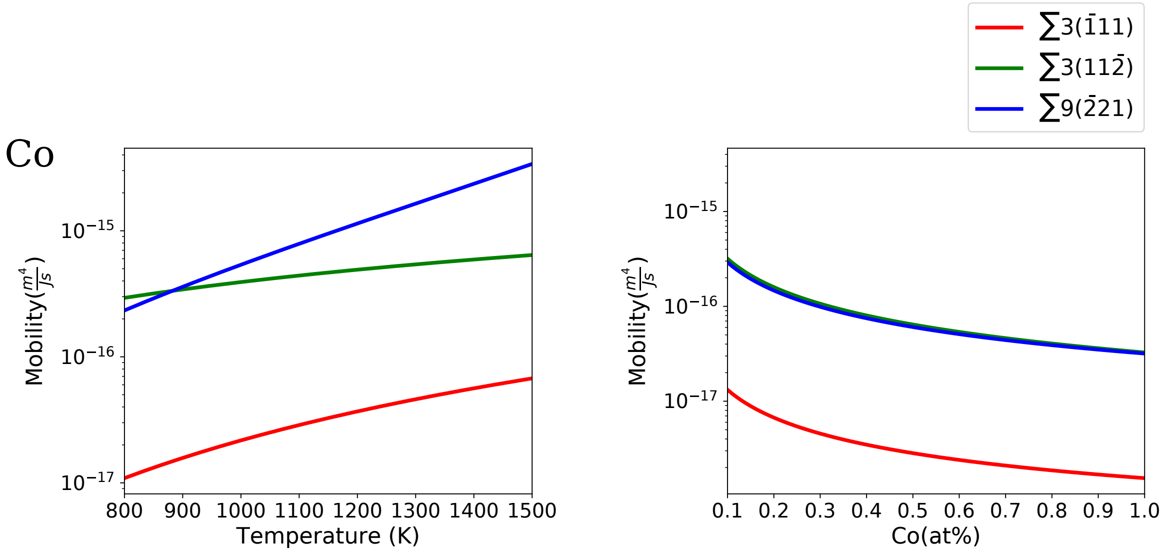


Figure S3: GB mobility as a function of temperature (left) at a fixed Co composition of 0.1 at.%, and as a function of Co composition (right) at a fixed temperature of 850 K.

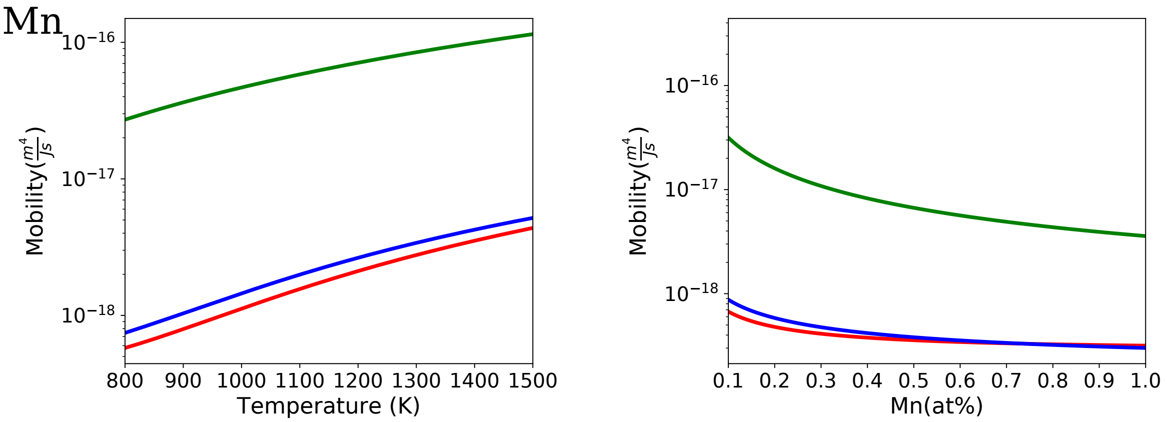


Figure S4: GB mobility as a function of temperature (left) at a fixed Mn composition of 0.1 at.%, and as a function of Mn composition (right) at a fixed temperature of 850 K.

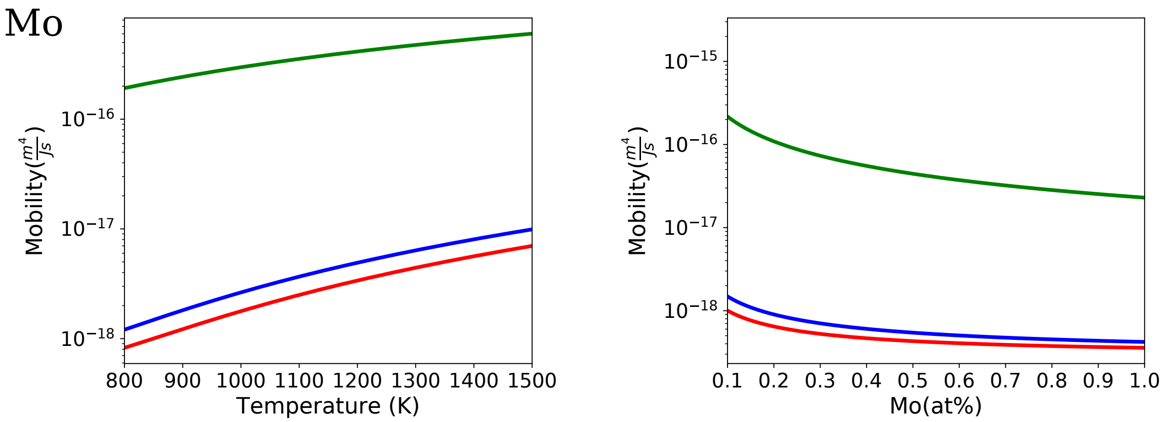


Figure S5: GB mobility as a function of temperature (left) at a fixed Mo composition of 0.1 at.%, and as a function of Mo composition (right) at a fixed temperature of 850 K.

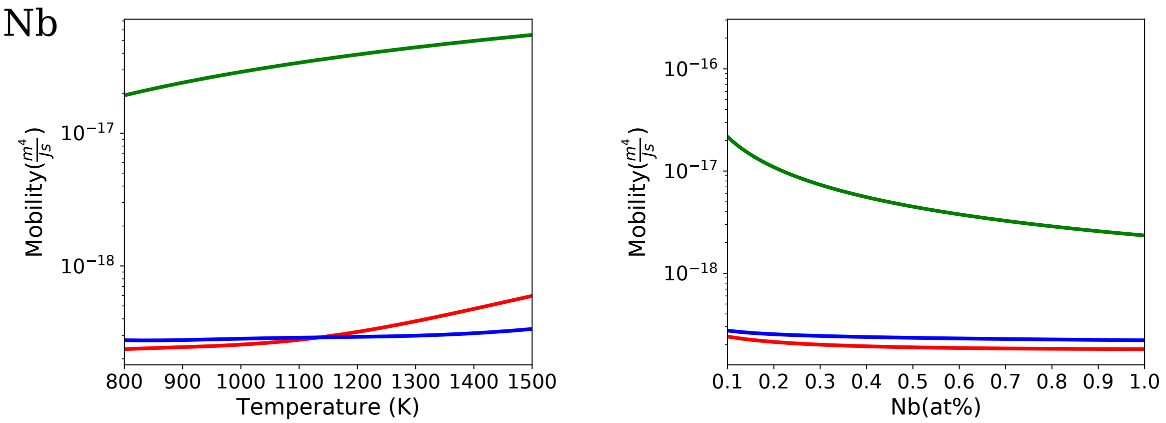


Figure S6: GB mobility as a function of temperature (left) at a fixed Nb composition of 0.1 at.%, and as a function of Nb composition (right) at a fixed temperature of 850 K.

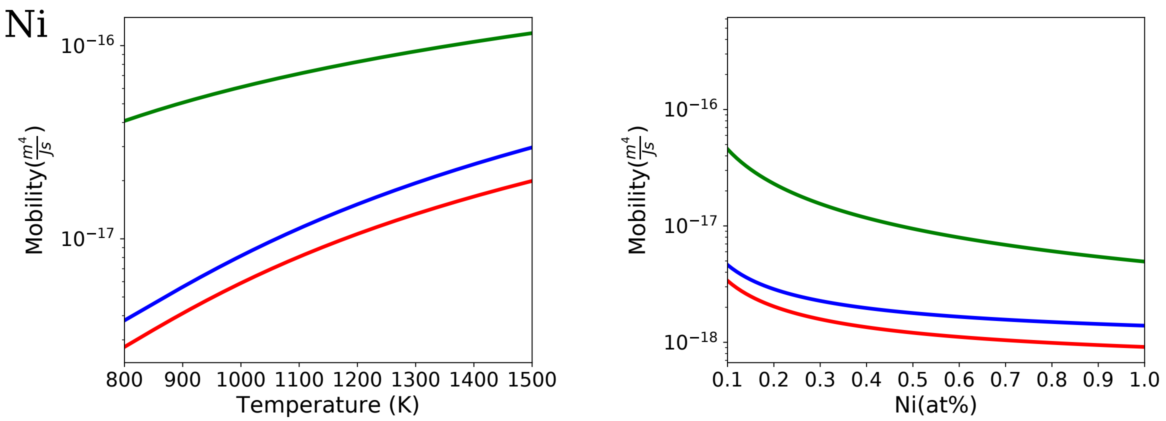


Figure S7: GB mobility as a function of temperature (left) at a fixed Ni composition of 0.1 at.%, and as a function of Ni composition (right) at a fixed temperature of 850 K.

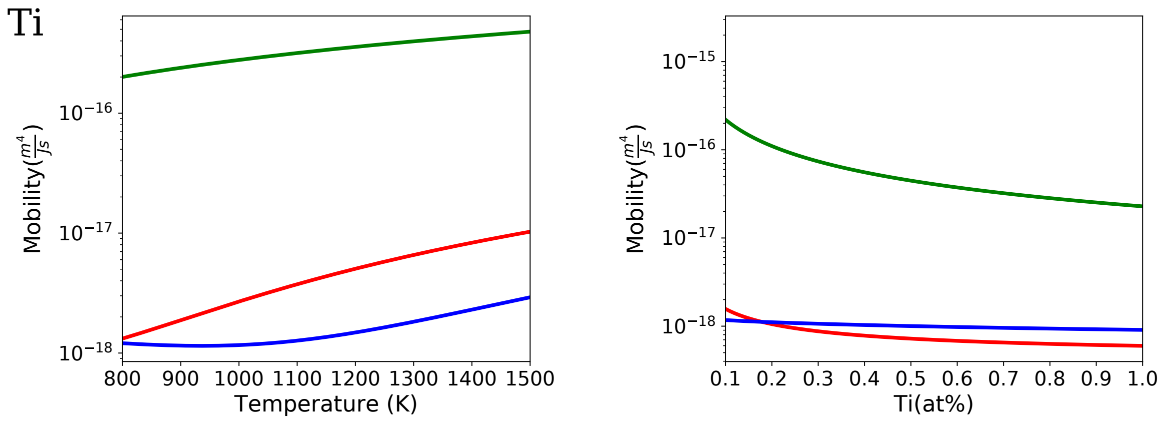


Figure S8: GB mobility as a function of temperature (left) at a fixed Ti composition of 0.1 at.%, and as a function of Ti composition (right) at a fixed temperature of 850 K.

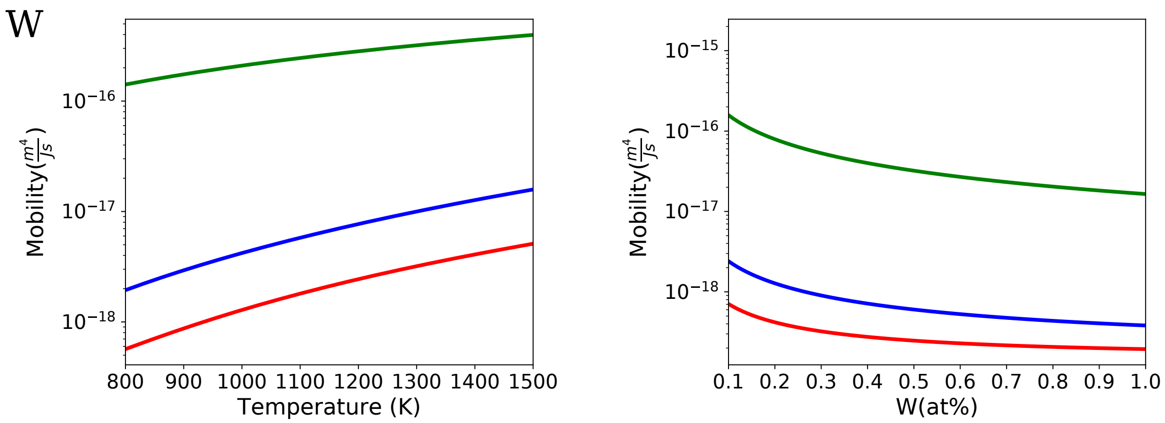


Figure S9: GB mobility as a function of temperature (left) at a fixed W composition of 0.1 at.%, and as a function of W composition (right) at a fixed temperature of 850 K.

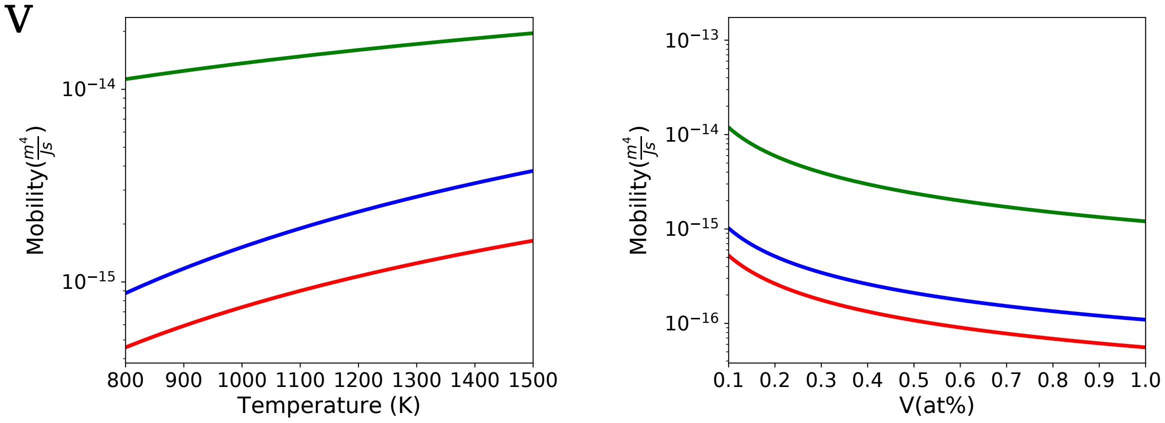


Figure S10: GB mobility as a function of temperature (left) at a fixed V composition of 0.1 at.%, and as a function of V composition (right) at a fixed temperature of 850 K.

## 4. Effect of GB energy and GB mobility

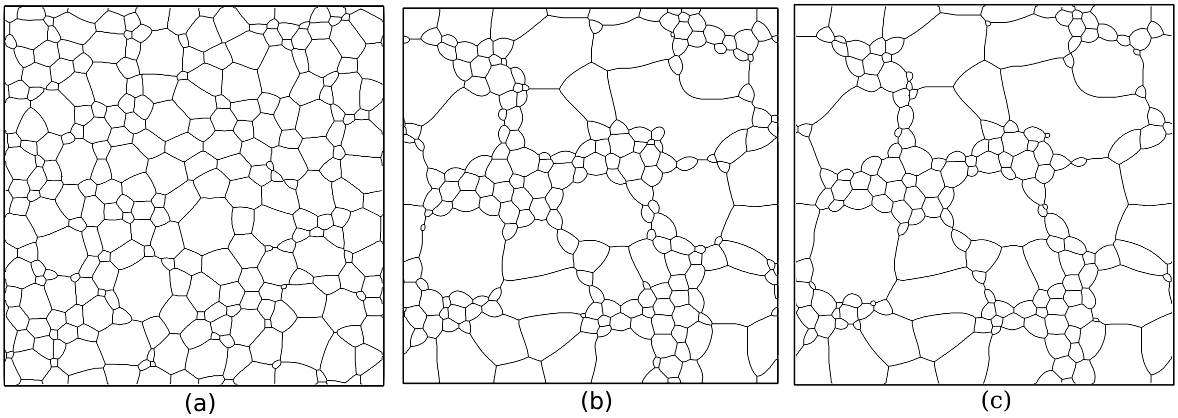


Figure S11: Effect of GB energy and mobility on microstructural evolution when considering a mixture of $\Sigma3$ $[110](11\bar{2})$ (10%) and $\Sigma9$ $[110](\bar{2}21)$ (90%) boundaries at 30000 timestep. The following conditions are analyzed: (a) Both GB types are assigned the same mobility (equal to the mobility of $\Sigma9$ $[110](\bar{2}21)$ boundary), but they have the actual GB energy. (b) Both GB types are assigned the same energy (equal to the energy of $\Sigma9$ $[110](\bar{2}21)$ boundary), but they have actual GB mobility. (c) The actual, distinct values of GB energy and GB mobility are retained for both boundary types. Clearly, the outcome depends on the choice of GB mobility.

## 5. Grain growth microstructure in the presence of different GB concentrations

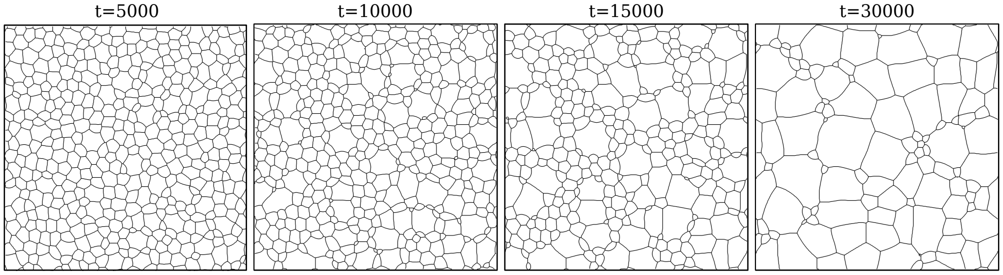


Figure S12: Grain growth behavior with Cr segregation for a mixture of grain boundaries. The boundary population includes 30% $\Sigma3$ [110](11$\bar{2}$) and 70% $\Sigma9$ [110]($\bar{2}$21) boundaries.

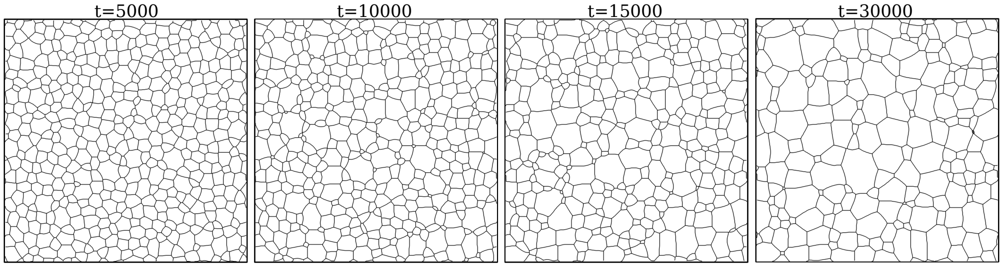


Figure S13: Grain growth behavior with Cr segregation for a mixture of grain boundaries. The boundary population includes 50% $\Sigma3$ [110](11$\bar{2}$) and 50% $\Sigma9$ [110]($\bar{2}$21) boundaries.

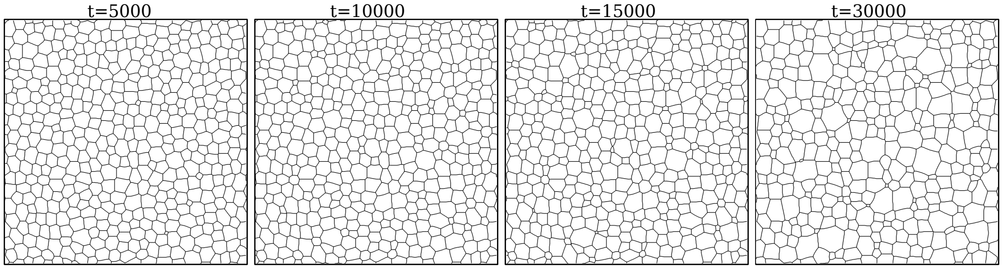


Figure S14: Grain growth behavior with Cr segregation for a mixture of grain boundaries. The boundary population includes 70% $\Sigma3$ [110](11$\bar{2}$) and 30% $\Sigma9$ [110]($\bar{2}$21) boundaries.

## References


[1] Y. Iijima, K. Kimura, C.-G. Lee, K. ichi Hirano, Impurity diffusion and isotope effect of cobalt in alpha;-iron, Materials Transactions, JIM 34 (1) (1993) 20–26. doi:10.2320/matertrans1989.34.20.

[2] C.-G. Lee, Y. Iijima, T. Hiratani, K. ichi Hirano, Diffusion of chromium in α-iron, Materials Transactions, JIM 31 (4) (1990) 255–261. doi:10.2320/matertrans1989.31.255.

[3] O. Hegde, V. Kulitckii, A. Schneider, F. Soisson, T. Hickel, J. Neugebauer, G. Wilde, S. Divinski, C.-C. Fu, Impact of magnetic transition on mn diffusion in $\alpha$-iron: Correlative state-of-the-art theoretical and experimental study, Phys. Rev. B 104 (2021) 184107. doi:10.1103/PhysRevB.104.184107. URL `https://link.aps.org/doi/10.1103/PhysRevB.104.184107`

[4] H. Nitta, T. Yamamoto, R. Kanno, K. Takasawa, T. Iida, Y. Yamazaki, S. Ogu, Y. Iijima, Diffusion of molybdenum in alpha-iron, Acta Materialia 50 (16) (2002) 4117–4125. doi:https://doi.org/10.1016/S1359-6454(02)00229-X. URL `https://www.sciencedirect.com/science/article/pii/S135964540200229X`

[5] N. Oono, H. Nitta, Y. Iijima, Diffusion of niobium in α-iron, MATERIALS TRANSACTIONS 44 (10) (2003) 2078–2083. doi:10.2320/matertrans.44.2078.

[6] J. Cermak, M. Lubbehusen, H. Mehrer, The influence of the magnetic phase transformation on the heterodiffusion of exp 63 ni in alpha-iron, Z. Metallkd. 80 (4) (1989) 213–219.

[7] P. Klugkist, C. Herzig, Tracer diffusion of titanium in alpha-iron, physica status solidi (a) 148 (2) (1995) 413–421. arXiv:https://onlinelibrary.wiley.com/doi/pdf/10.1002/pssa.2211480209, doi:https://doi.org/10.1002/pssa.2211480209. URL `https://onlinelibrary.wiley.com/doi/abs/10.1002/pssa.2211480209`

[8] S. Takemoto, H. Nitta, Y. Iijima, Y. Yamazaki, Diffusion of tungsten in alpha-iron, Philosophical Magazine 87 (11) (2007) 1619–1629. doi:10.1080/14786430600732093.

[9] C. D. Versteylen, N. H. van Dijk, M. H. F. Sluiter, First-principles analysis of solute diffusion in dilute bcc fe-$X$ alloys, Phys. Rev. B 96 (2017) 094105. doi:10.1103/PhysRevB.96.094105. URL `https://link.aps.org/doi/10.1103/PhysRevB.96.094105`
